# Supplementary material for: Seeing and Reasoning with Confidence: Supercharging Multimodal LLMs with an Uncertainty-Aware Agentic Framework
Source: arXiv:2503.08308 source file (2025-03-11)

Stage1

Stage2

**Q1:** What color is a man's hair?

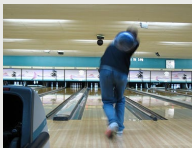

**GT:** Black.  
**MLLM:** Blue.

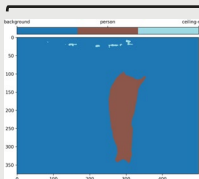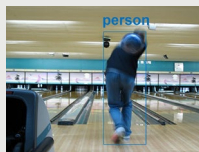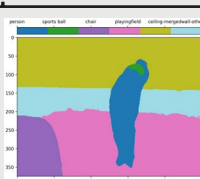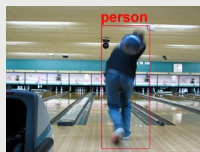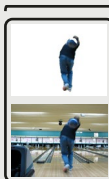

**A\*:** Black.  
( $US = 2.5$ )

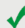

**A:** Blue.  
( $US = 2.9$ )

**Q2:** What color is the hand of the captain of the toy plane?

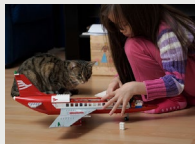

**GT:** Yellow.  
**MLLM:** White.

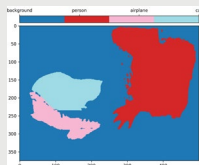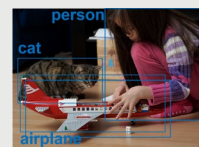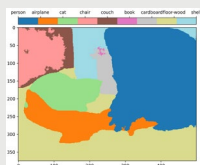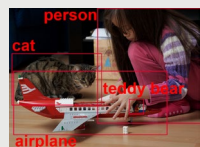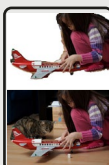

**A:** White.  
( $US = 1.9$ )

**A:** Yellow.  
( $US = 1.3$ )

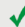

**Q3:** What is in the image?

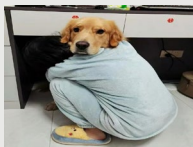

**GT:** A dog and a person.  
**MLLM:** A dog.

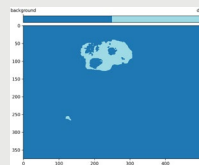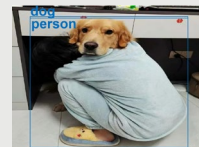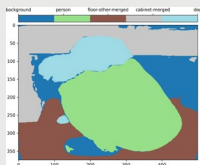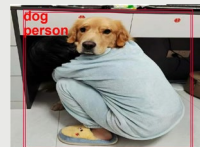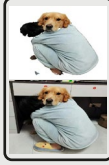

**A\*:** A dog and a person.  
( $US = 2.8$ )

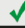

**A:** A dog and a person.  
( $US = 3.7$ )

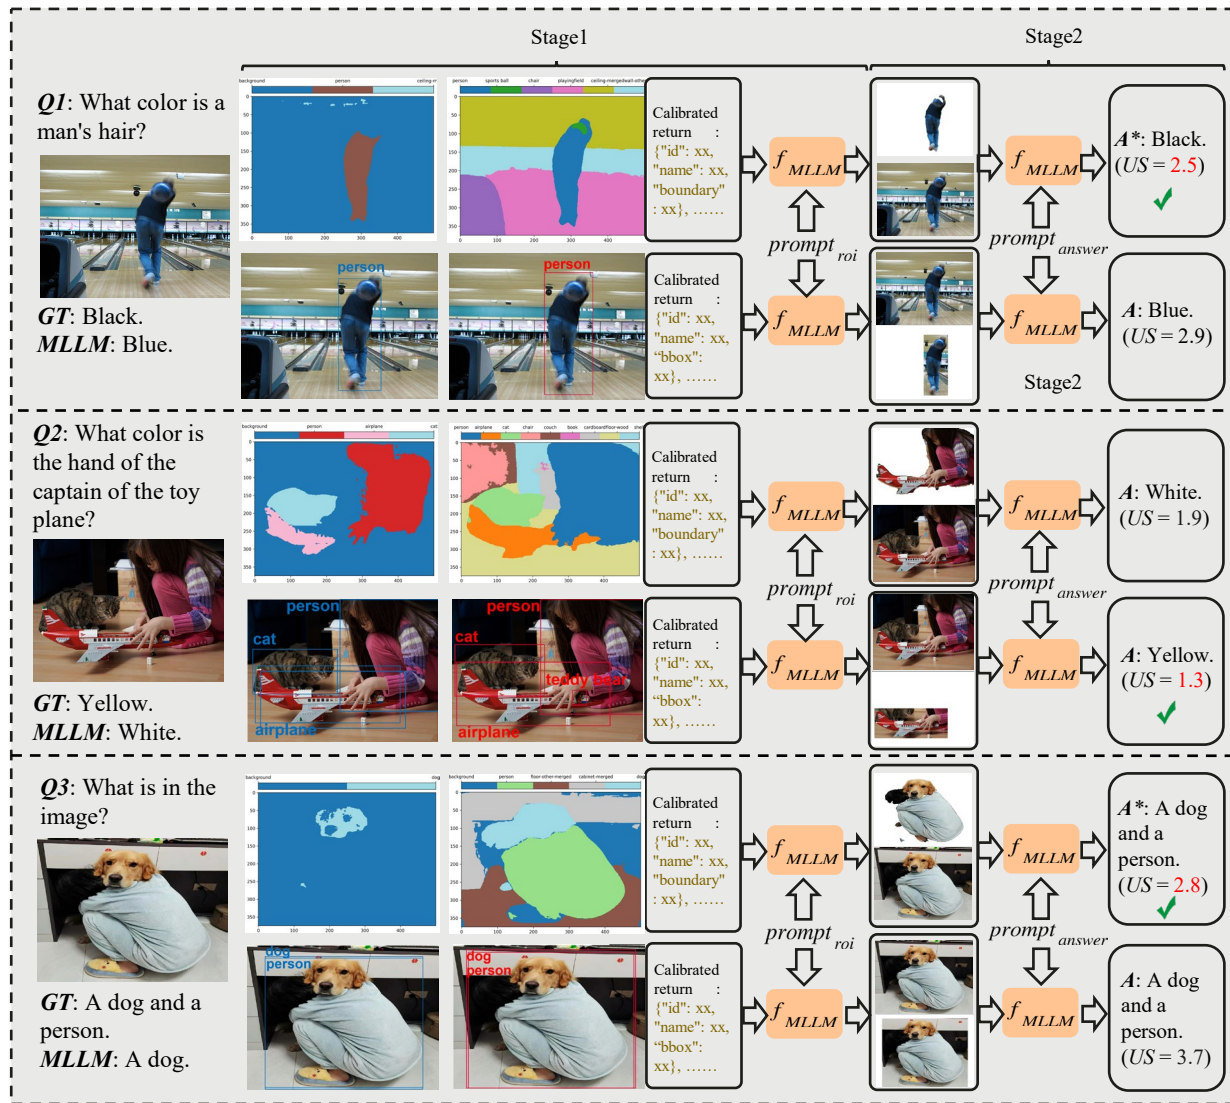

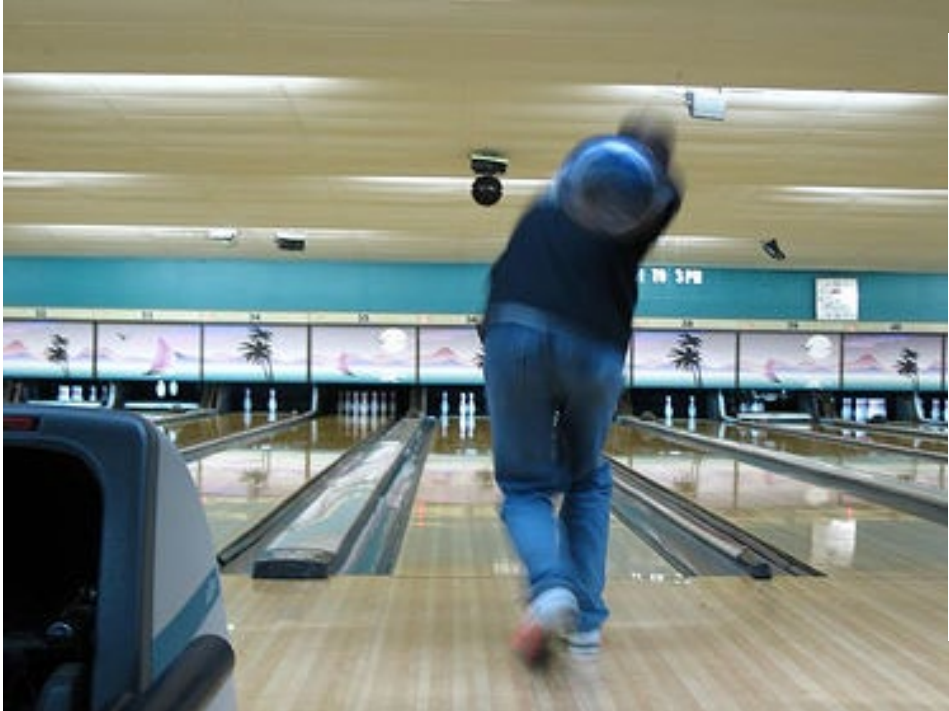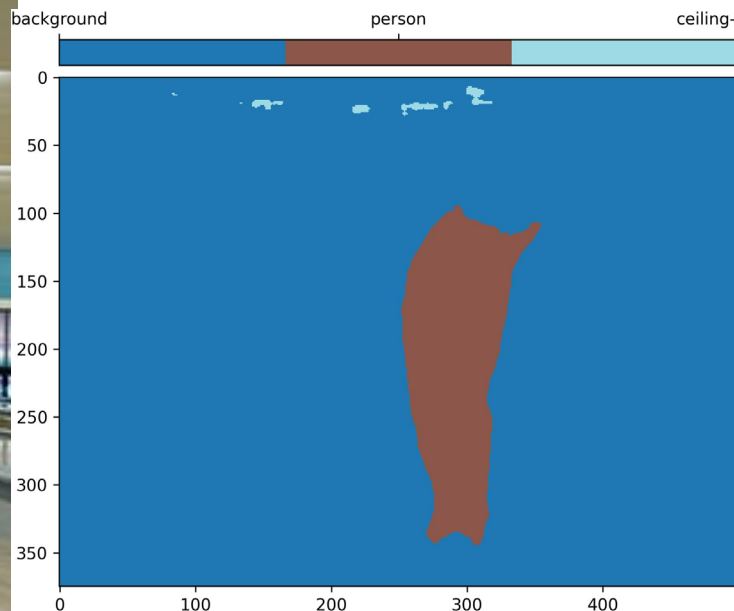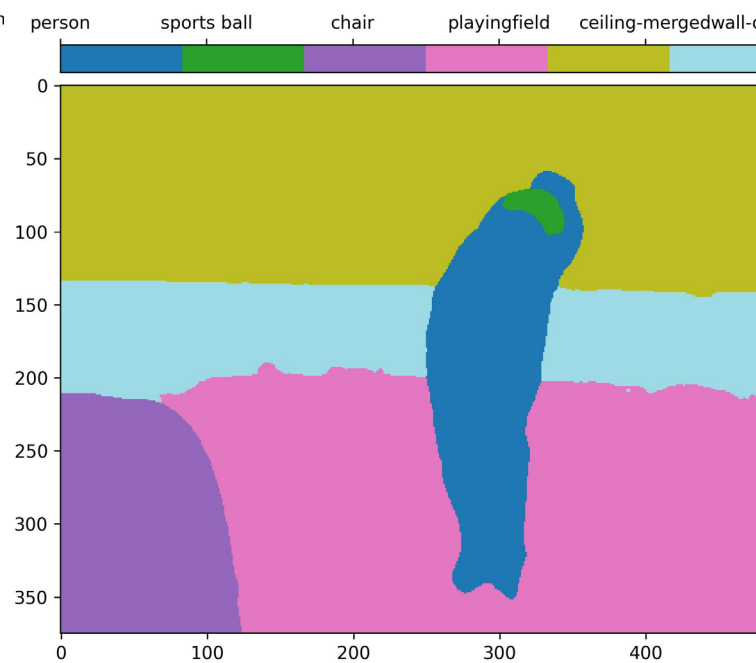

:  
 what is the color of man's hair, black  
 or blue?

MLLM: BLUE X what is the color of  
 man's hair, black or blue?

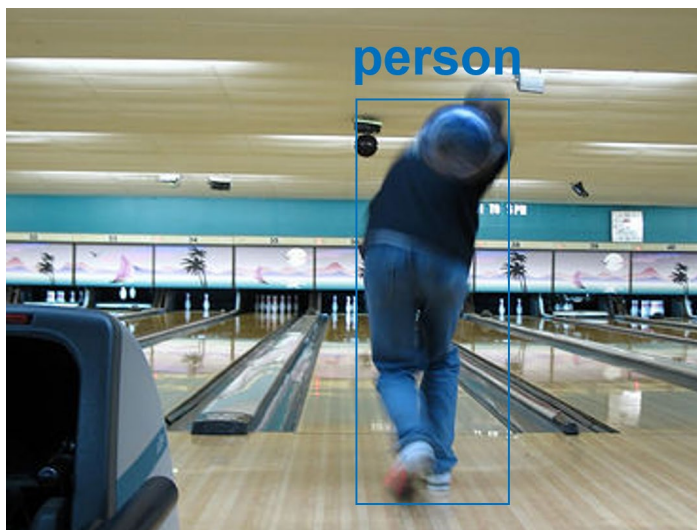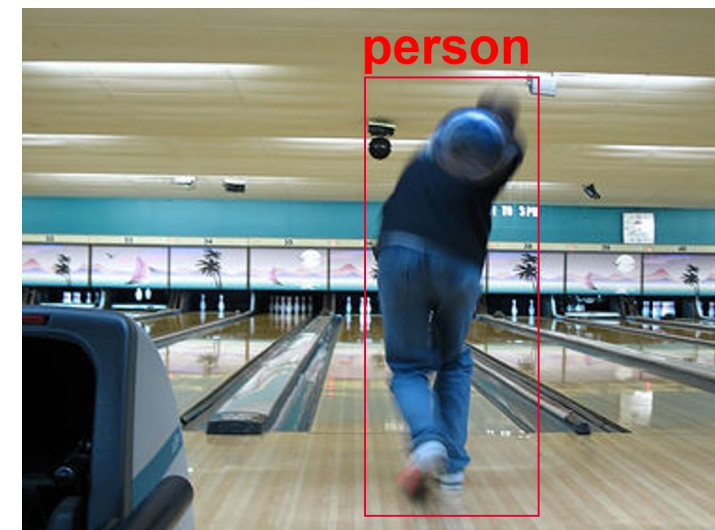

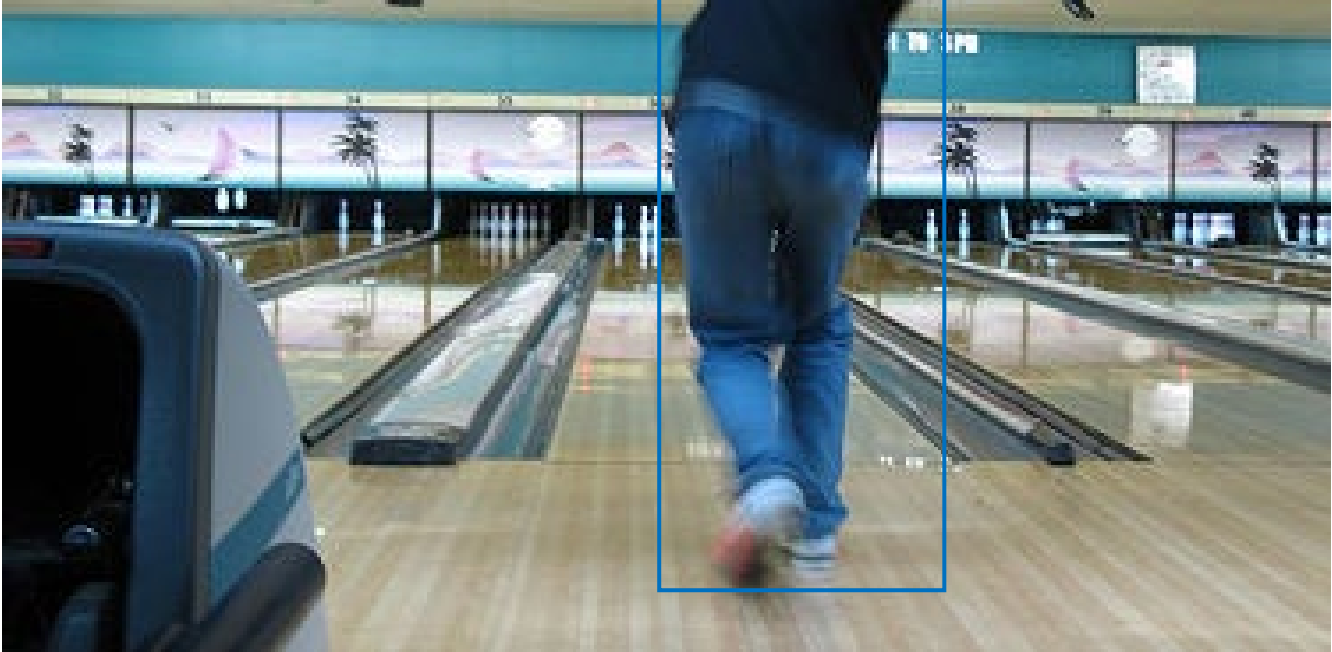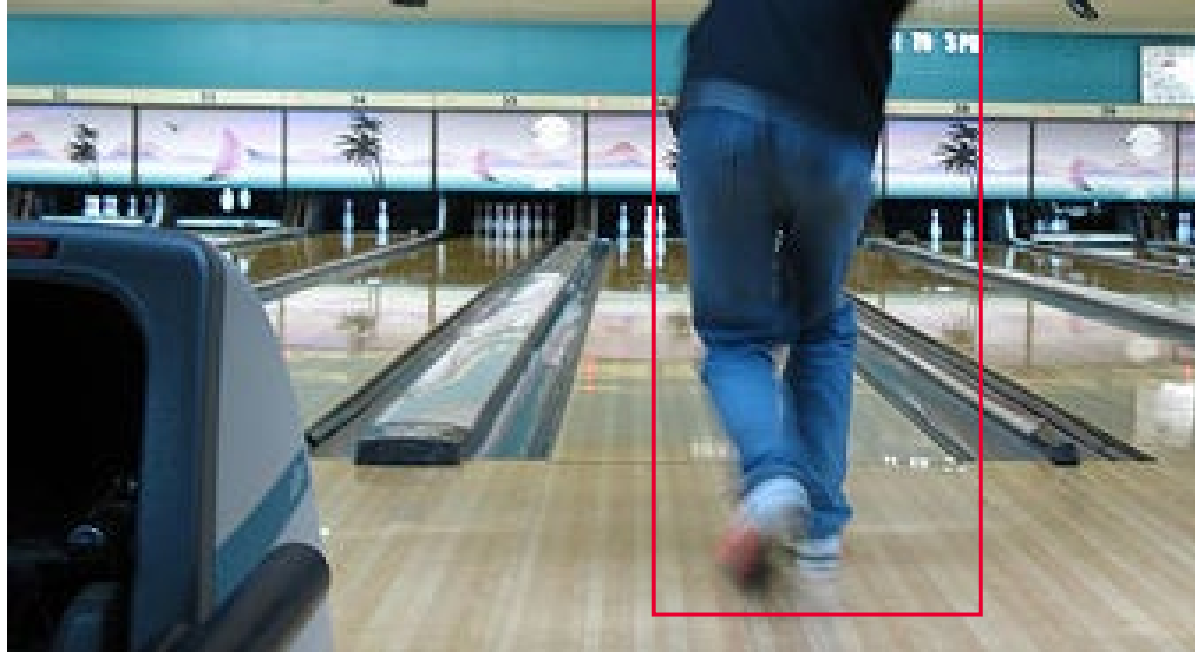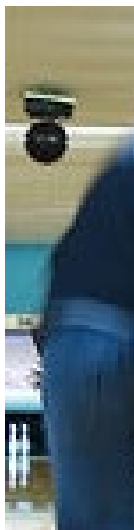



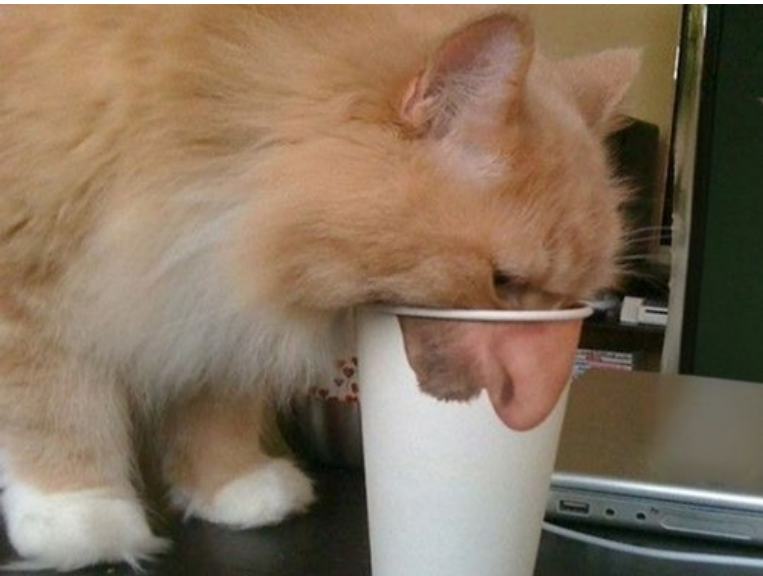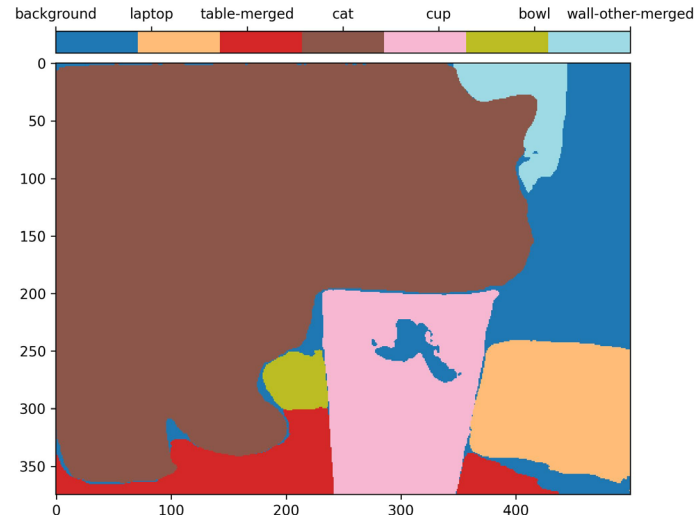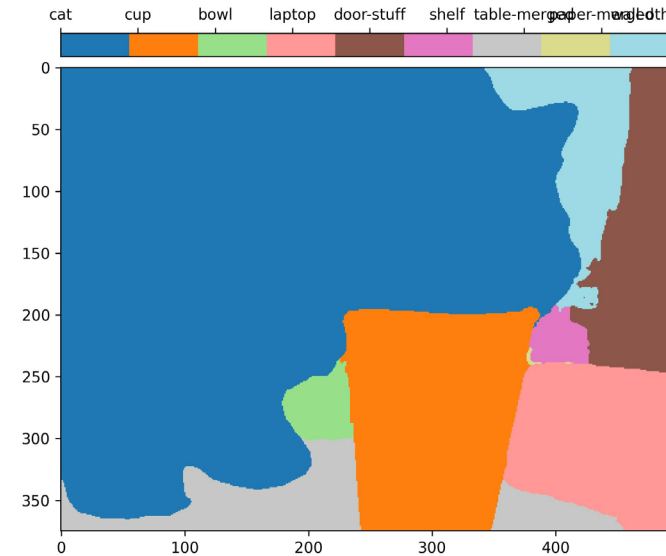

What is the color of  
the cat's nose?

GT: unanswerable

MLLM: Pink

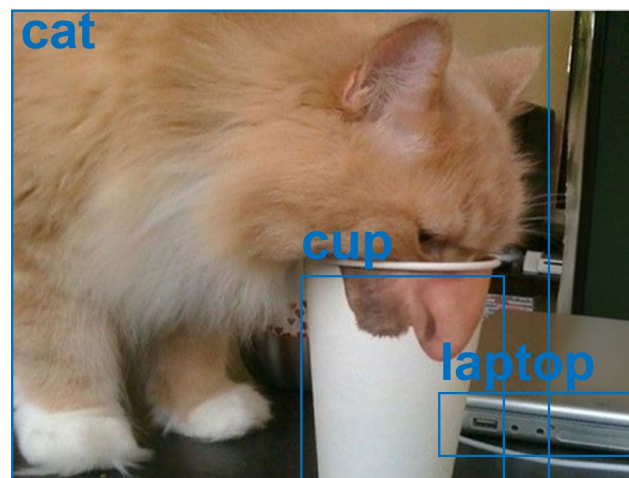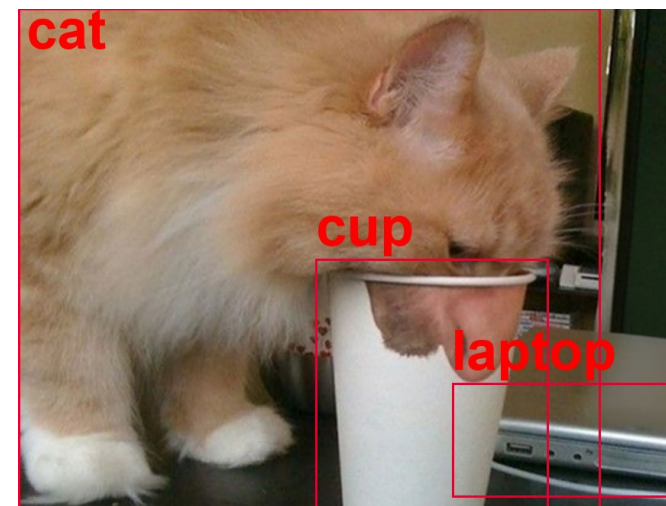

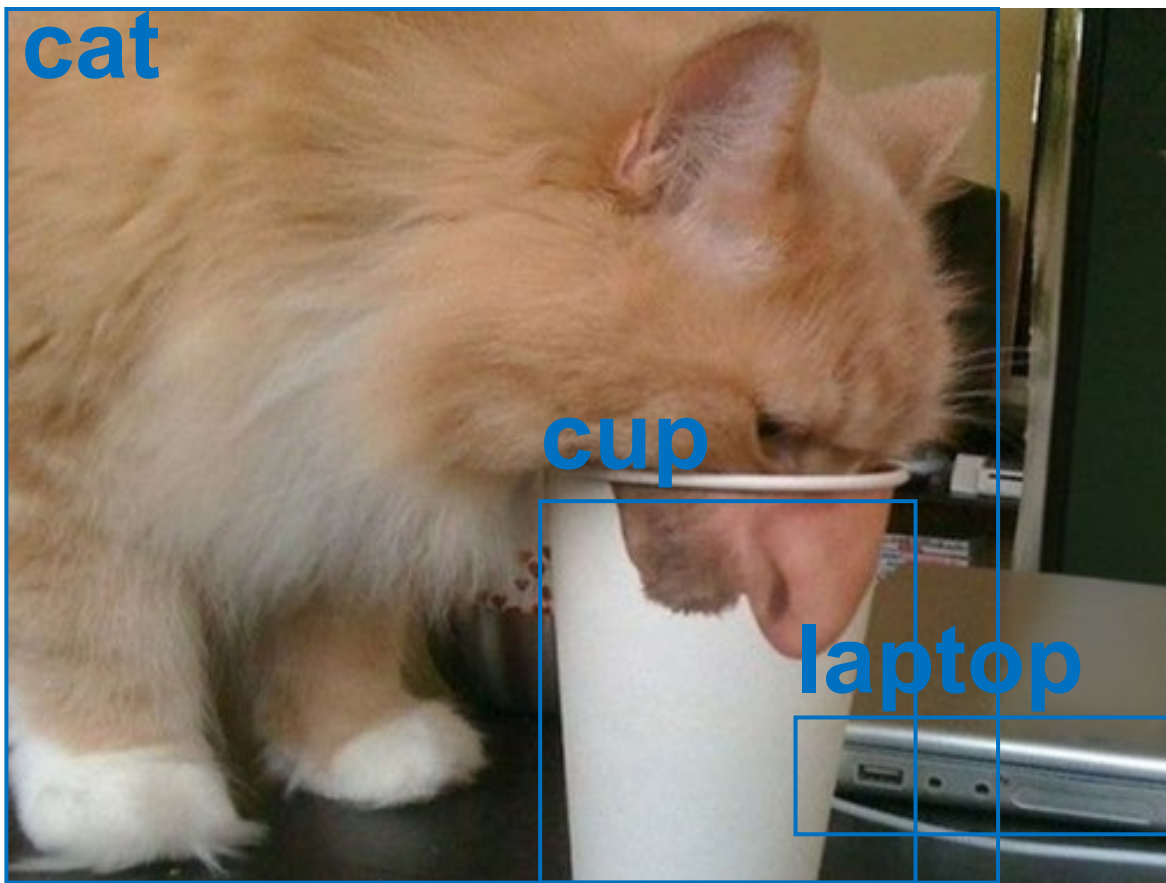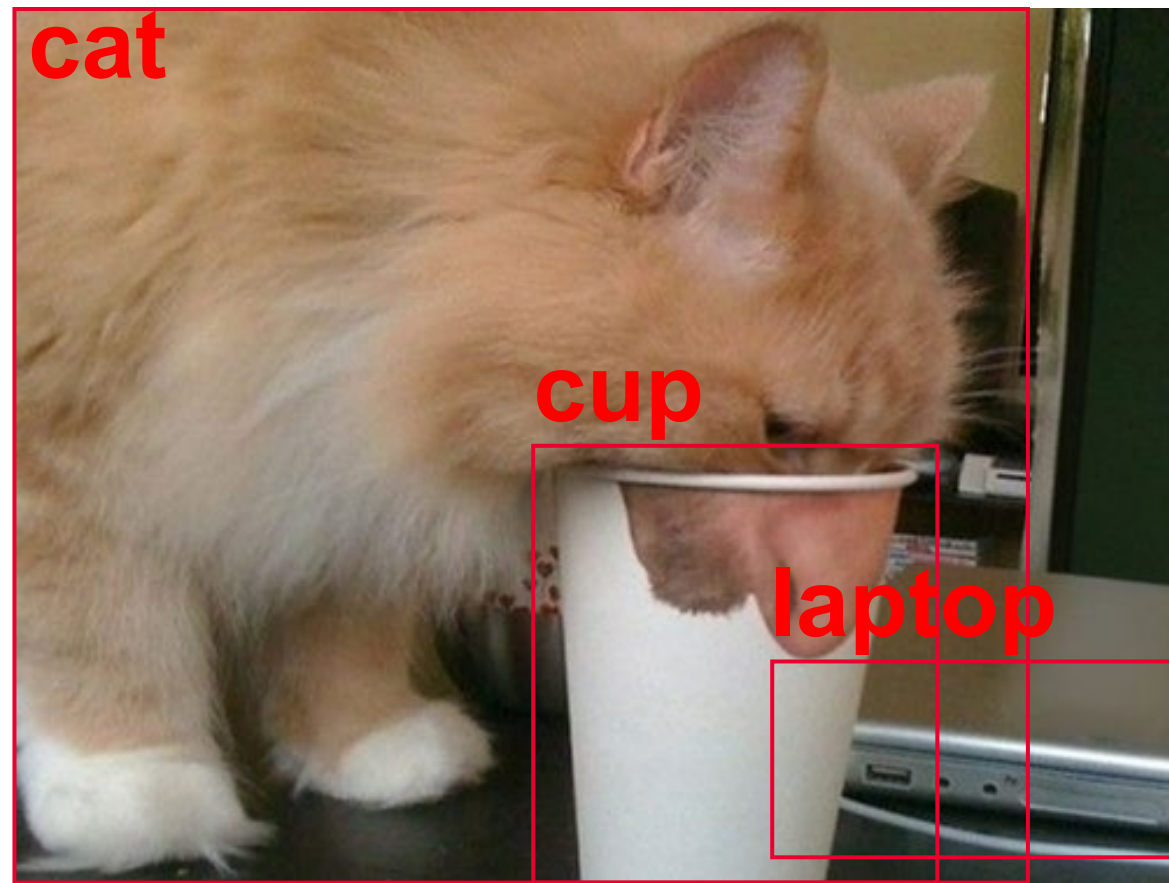



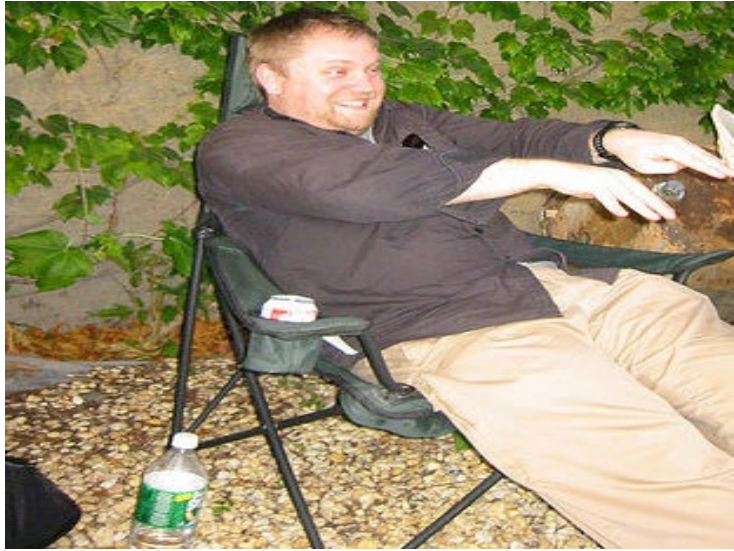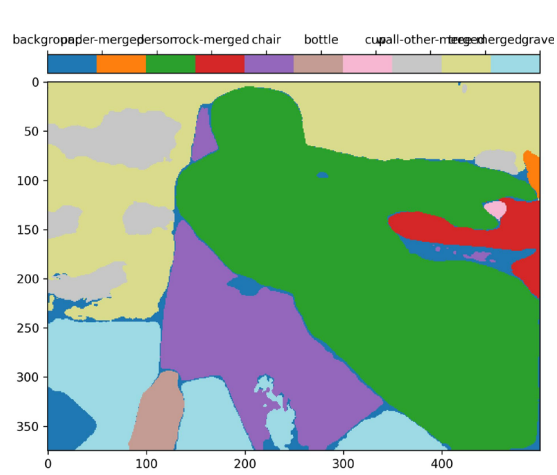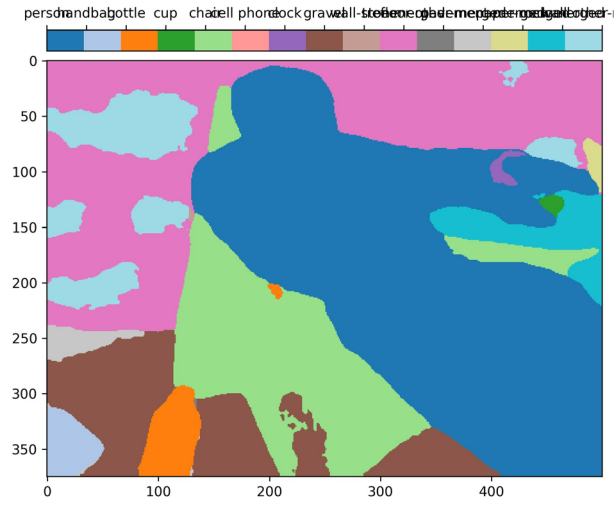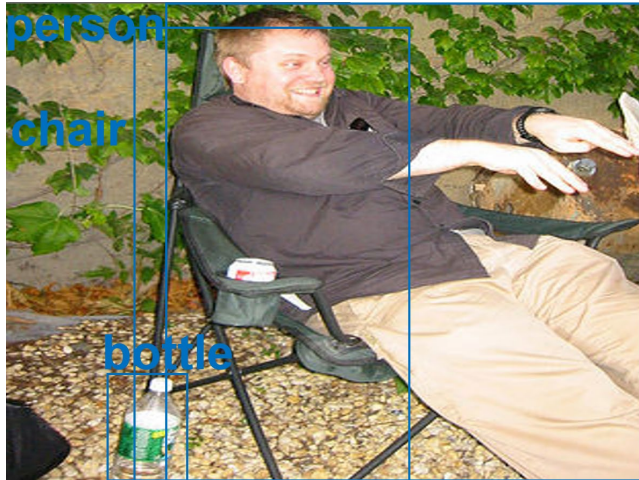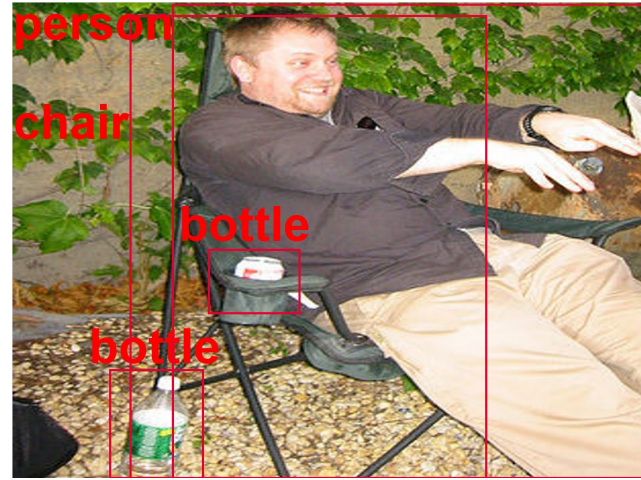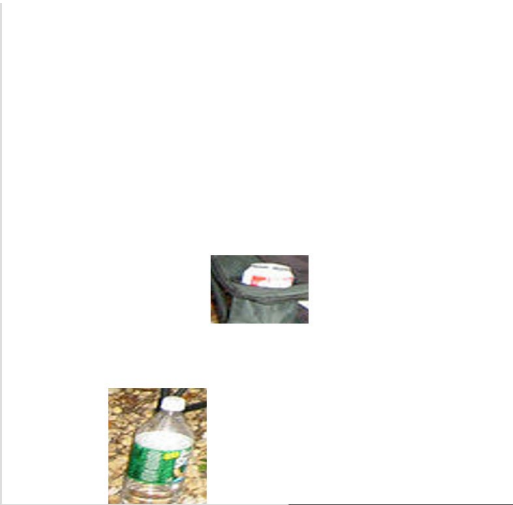

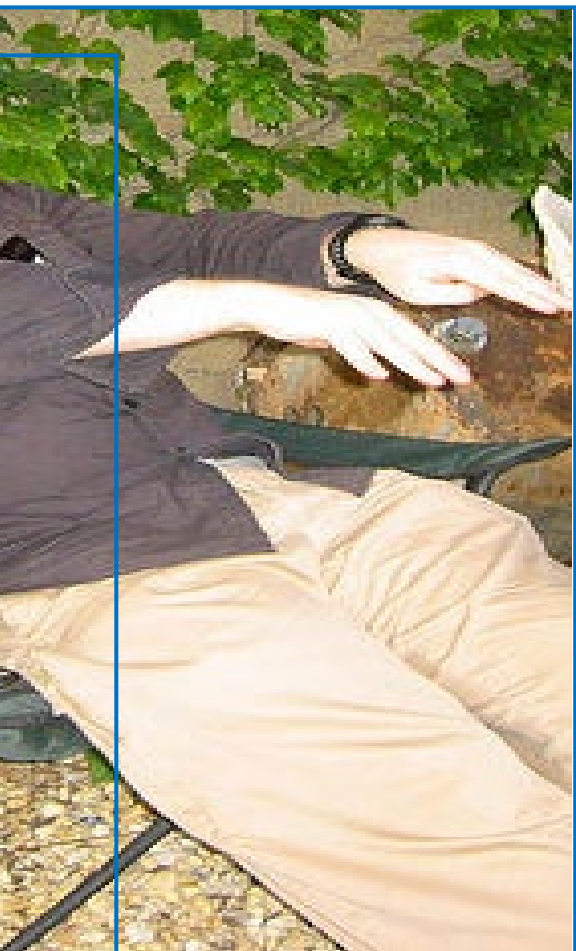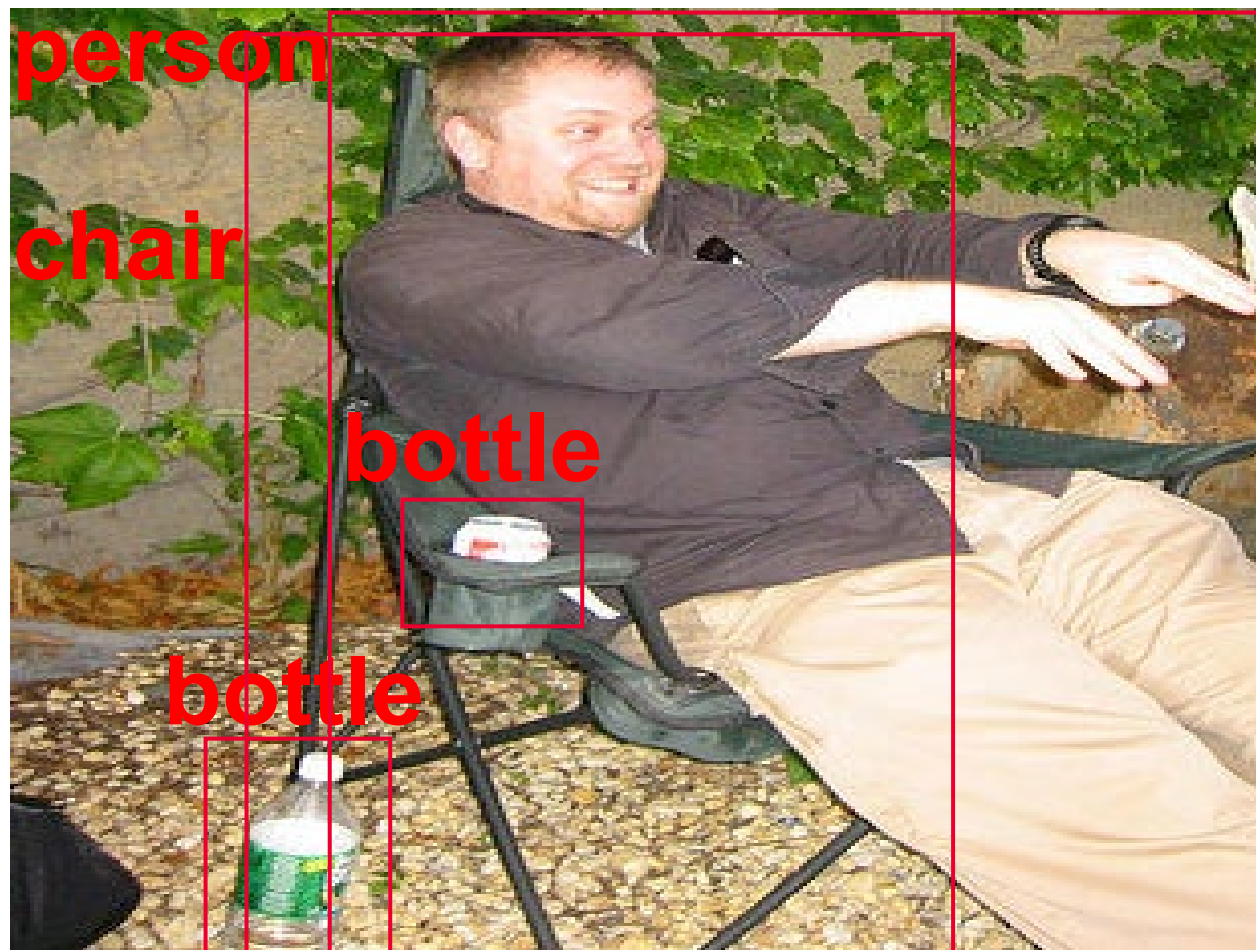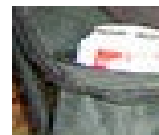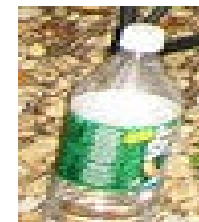

Supplement: Supplementary file 1 [file visual_appendix.pdf]
